# Supplementary material for: Nearly perfect sequences with arbitrary out-of-phase autocorrelation
Source: arXiv:1408.6883 source file (2014-09-02)
Supplement: Supplementary file 1 [file DPDS-appendix.tex]

\newpage
\appendix
\section{Tables }
%\twocolumn
%p{0.64\textwidth}

\begin{multicols}{2}

\setbox\ltmcbox\vbox{
\makeatletter\col@number\@ne
\tiny
% [inline block 0: 8 envs, 80985 chars -> data_tex | \begin{longtable}{|l|l|l|} \caption[m-ary]{$p$-ary nearly perfect sequences of period $n$ and type  $\gamma = 0$.}...]


\unskip
\unpenalty
\unpenalty
}

\unvbox\ltmcbox

\end{multicols}
